# Supplementary material for: Curriculum Learning Strategies for IR: An Empirical Study on Conversation Response Ranking
Source: arXiv:1912.08555 source file (2019-12-18)
Supplement: Supplementary file 1 [file 7_appendix.tex]

\section*{Appendix}

%\input{sections/table-difficulty.tex}

% \begin{figure}[h]
%     \centering
%     \includegraphics[width=0.60\textwidth]{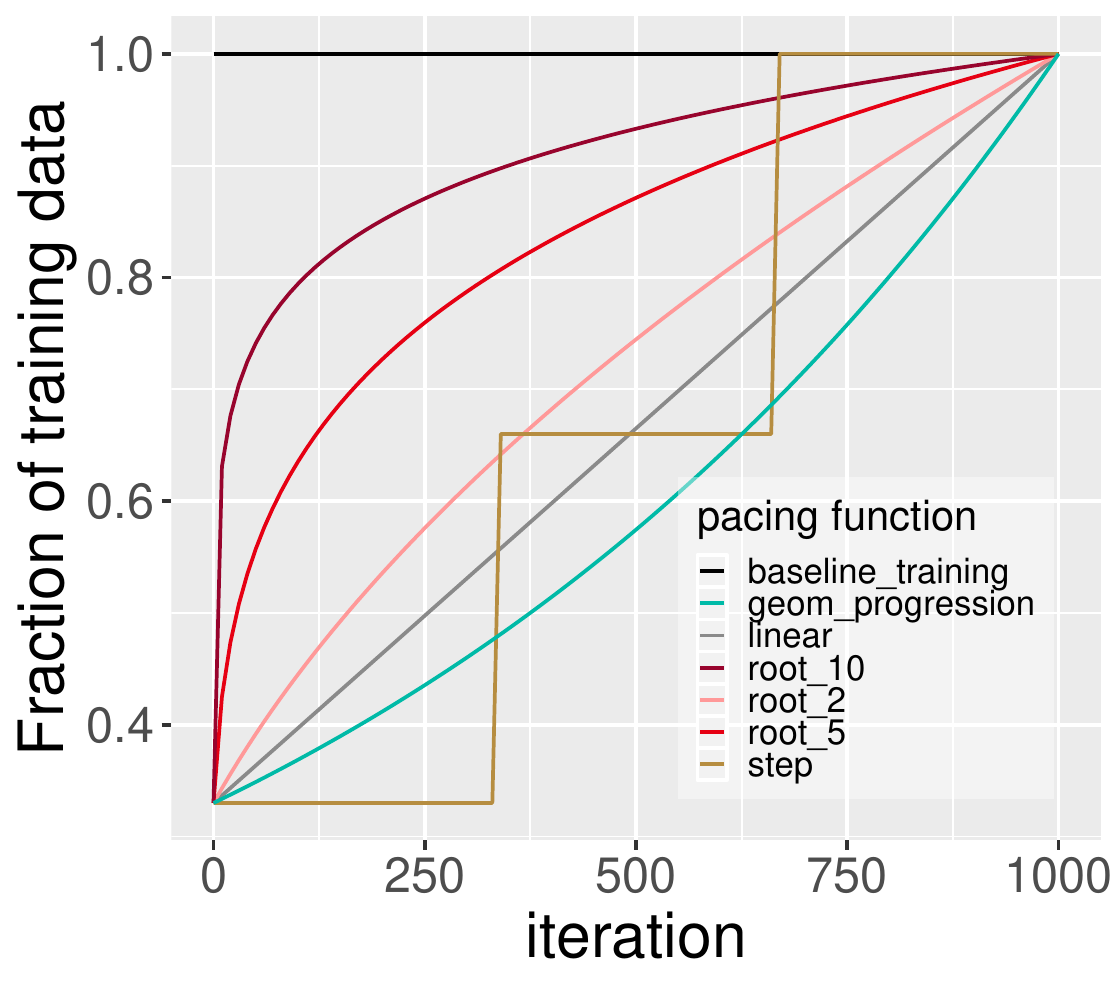}
%     \caption{Pacing functions example with initial dataset size $c_0=0.33$ and total number of curriculum learning iterations $T=1000$.
%     }
%     \label{fig:pacing_functions}
% \end{figure}

\subsubsection{\avgnumwordsd in \mantis{}}
If we use a simple word matching heuristic to identify noisy instances, Table~\ref{table:noisy_examples}, we see that \msdialog{} has a lower percentage ($\sim$ 3\%) of uninformative and noisy test set dialogues within the first $33\%$ instances ordered by \avgnumwordsd, compared to the $\sim$ 15\% of \mantis{}. This happens due to a practice of editing previous answers in StackExchange that does not happen in the Microsoft Technical Forum. Artifacts of the dataset can render manually defined scoring functions, such as \avgnumwordsd, obsolete for curriculum learning.

\begin{table}[h!]
\centering
\caption{Examples of noisy instances from the test set of the datasets, where the answer is uninformative and all the candidate responses have the same purpose, including the negative sampled ones (label equal 0).}
\label{table:noisy_examples}
\begin{tabular}{@{}ll@{}}
\toprule
\textbf{Label} & \multicolumn{1}{c}{\textbf{Example of noisy instance - $\set{R}_i$ for a fixed $\set{U}_i$}} \\ \midrule
\multicolumn{2}{c}{Extracted from \textbf{\mantis{} }} \\ \midrule
1 & I updated my answer a little pls check it again \\
0 & I updated my answer, windows use DOS format [...] \\
0 & \texttt{USER} I have just added a link at the end of my answer go and check it \\
0 & \texttt{USER} updated answer \\
0 & \texttt{USER} please check my answer as the correct if you think like that. Thanks. \\ \midrule \multicolumn{2}{c}{Extracted from \textbf{\msdialog{}}} \\ \midrule
1 & You are welcome \\
0 & Hi \texttt{USER} You are very welcome! Regards \texttt{USER}, Bing Ads Support Engineer \\
0 & You're welcome and thanks for the feedback. \\
0 & You're welcome. \texttt{USER} for the incovenience \\
0 & You're quite welcome \\ \midrule
\end{tabular}
\end{table}

\begin{figure}[h]
    \centering
    \includegraphics[width=0.9\textwidth]{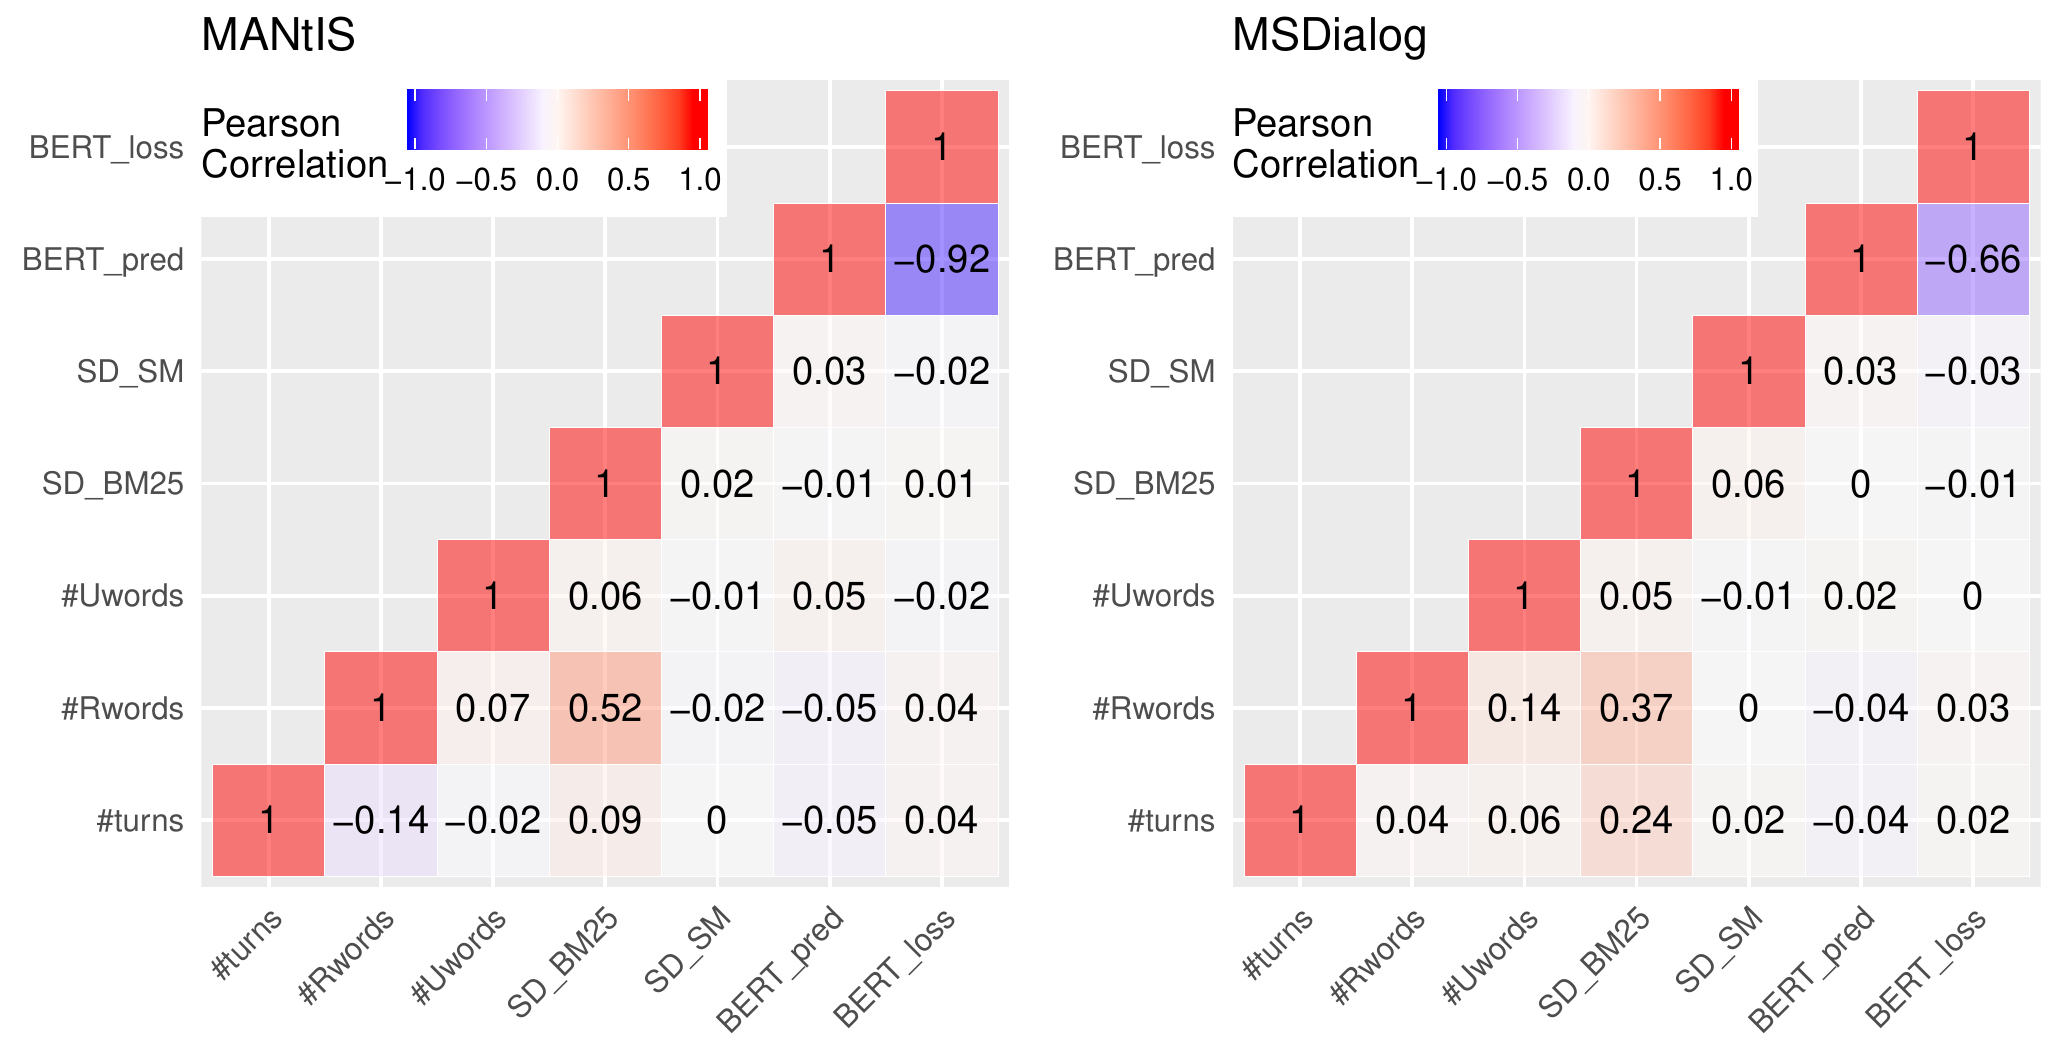}
    \caption{Correlation between scoring functions. The BERT based scoring functions have high correlation between them and low correlation with the manually defined ones.}
    \label{fig:corr_scoring}
\end{figure}

\begin{figure}[h]
    \centering
    \includegraphics[width=0.9\textwidth]{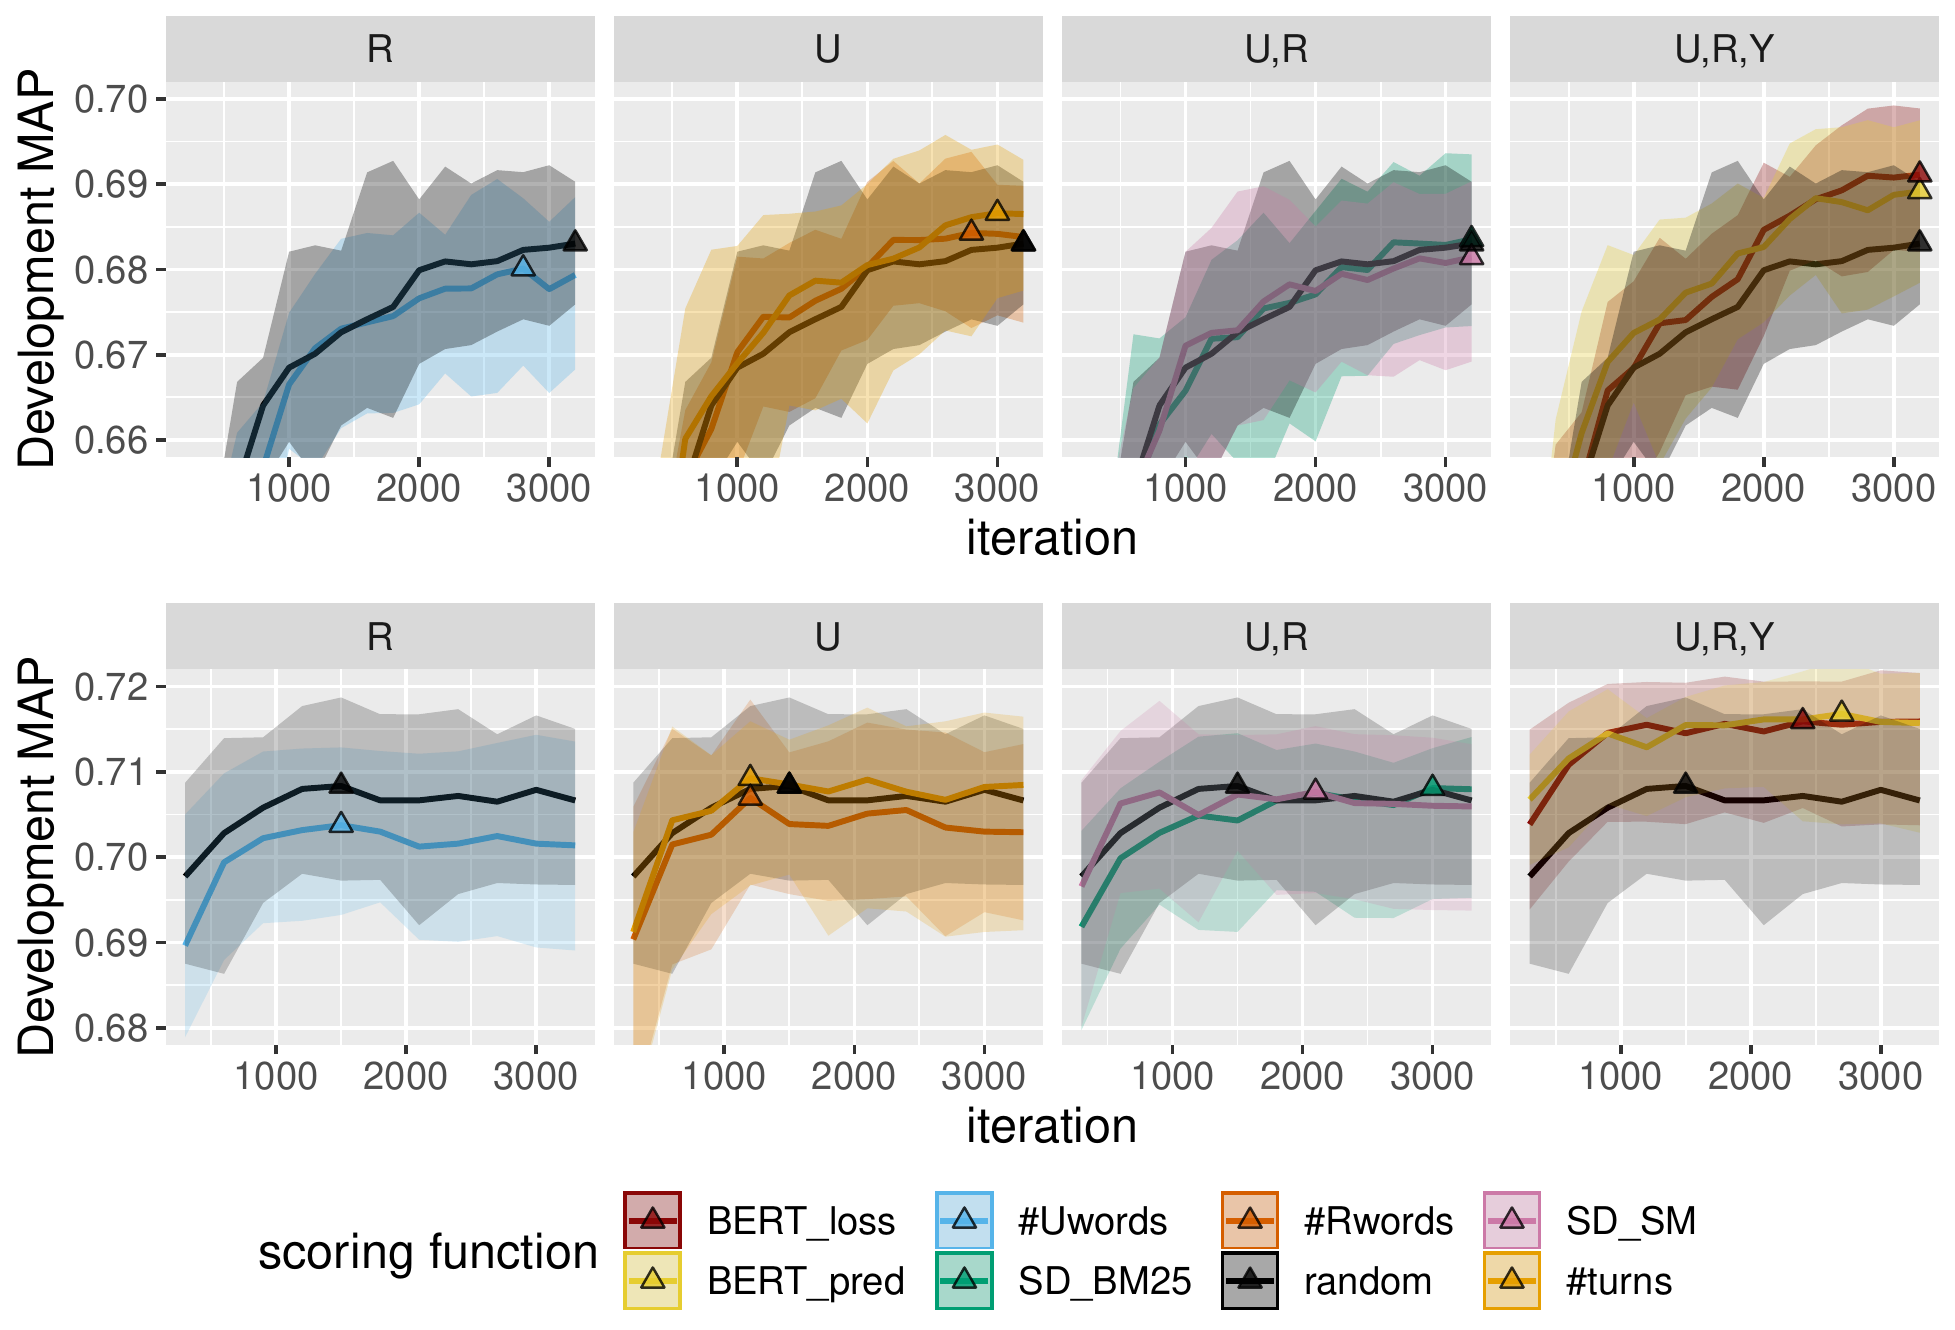}
    \caption{Average development MAP (strong lines) for 5 different runs of fine tuning BERT for conversation response ranking using different curriculum scoring functions. The top and bottom of the polygon around the strong line indicate the maximum and minimum values respectively, observed at each iteration, and $\bigtriangleup$ indicates the maximum MAP over all values observed during training. The black lines are the baseline where the scoring function is the $random$ scoring function. We fix the pacing function $p(t)$ as \textit{root\_2}}
    \label{fig:results_scoring}
\end{figure}

\begin{figure}
\centering
\begin{subfigure}{.5\textwidth}
  \centering
  \includegraphics[width=1\textwidth]{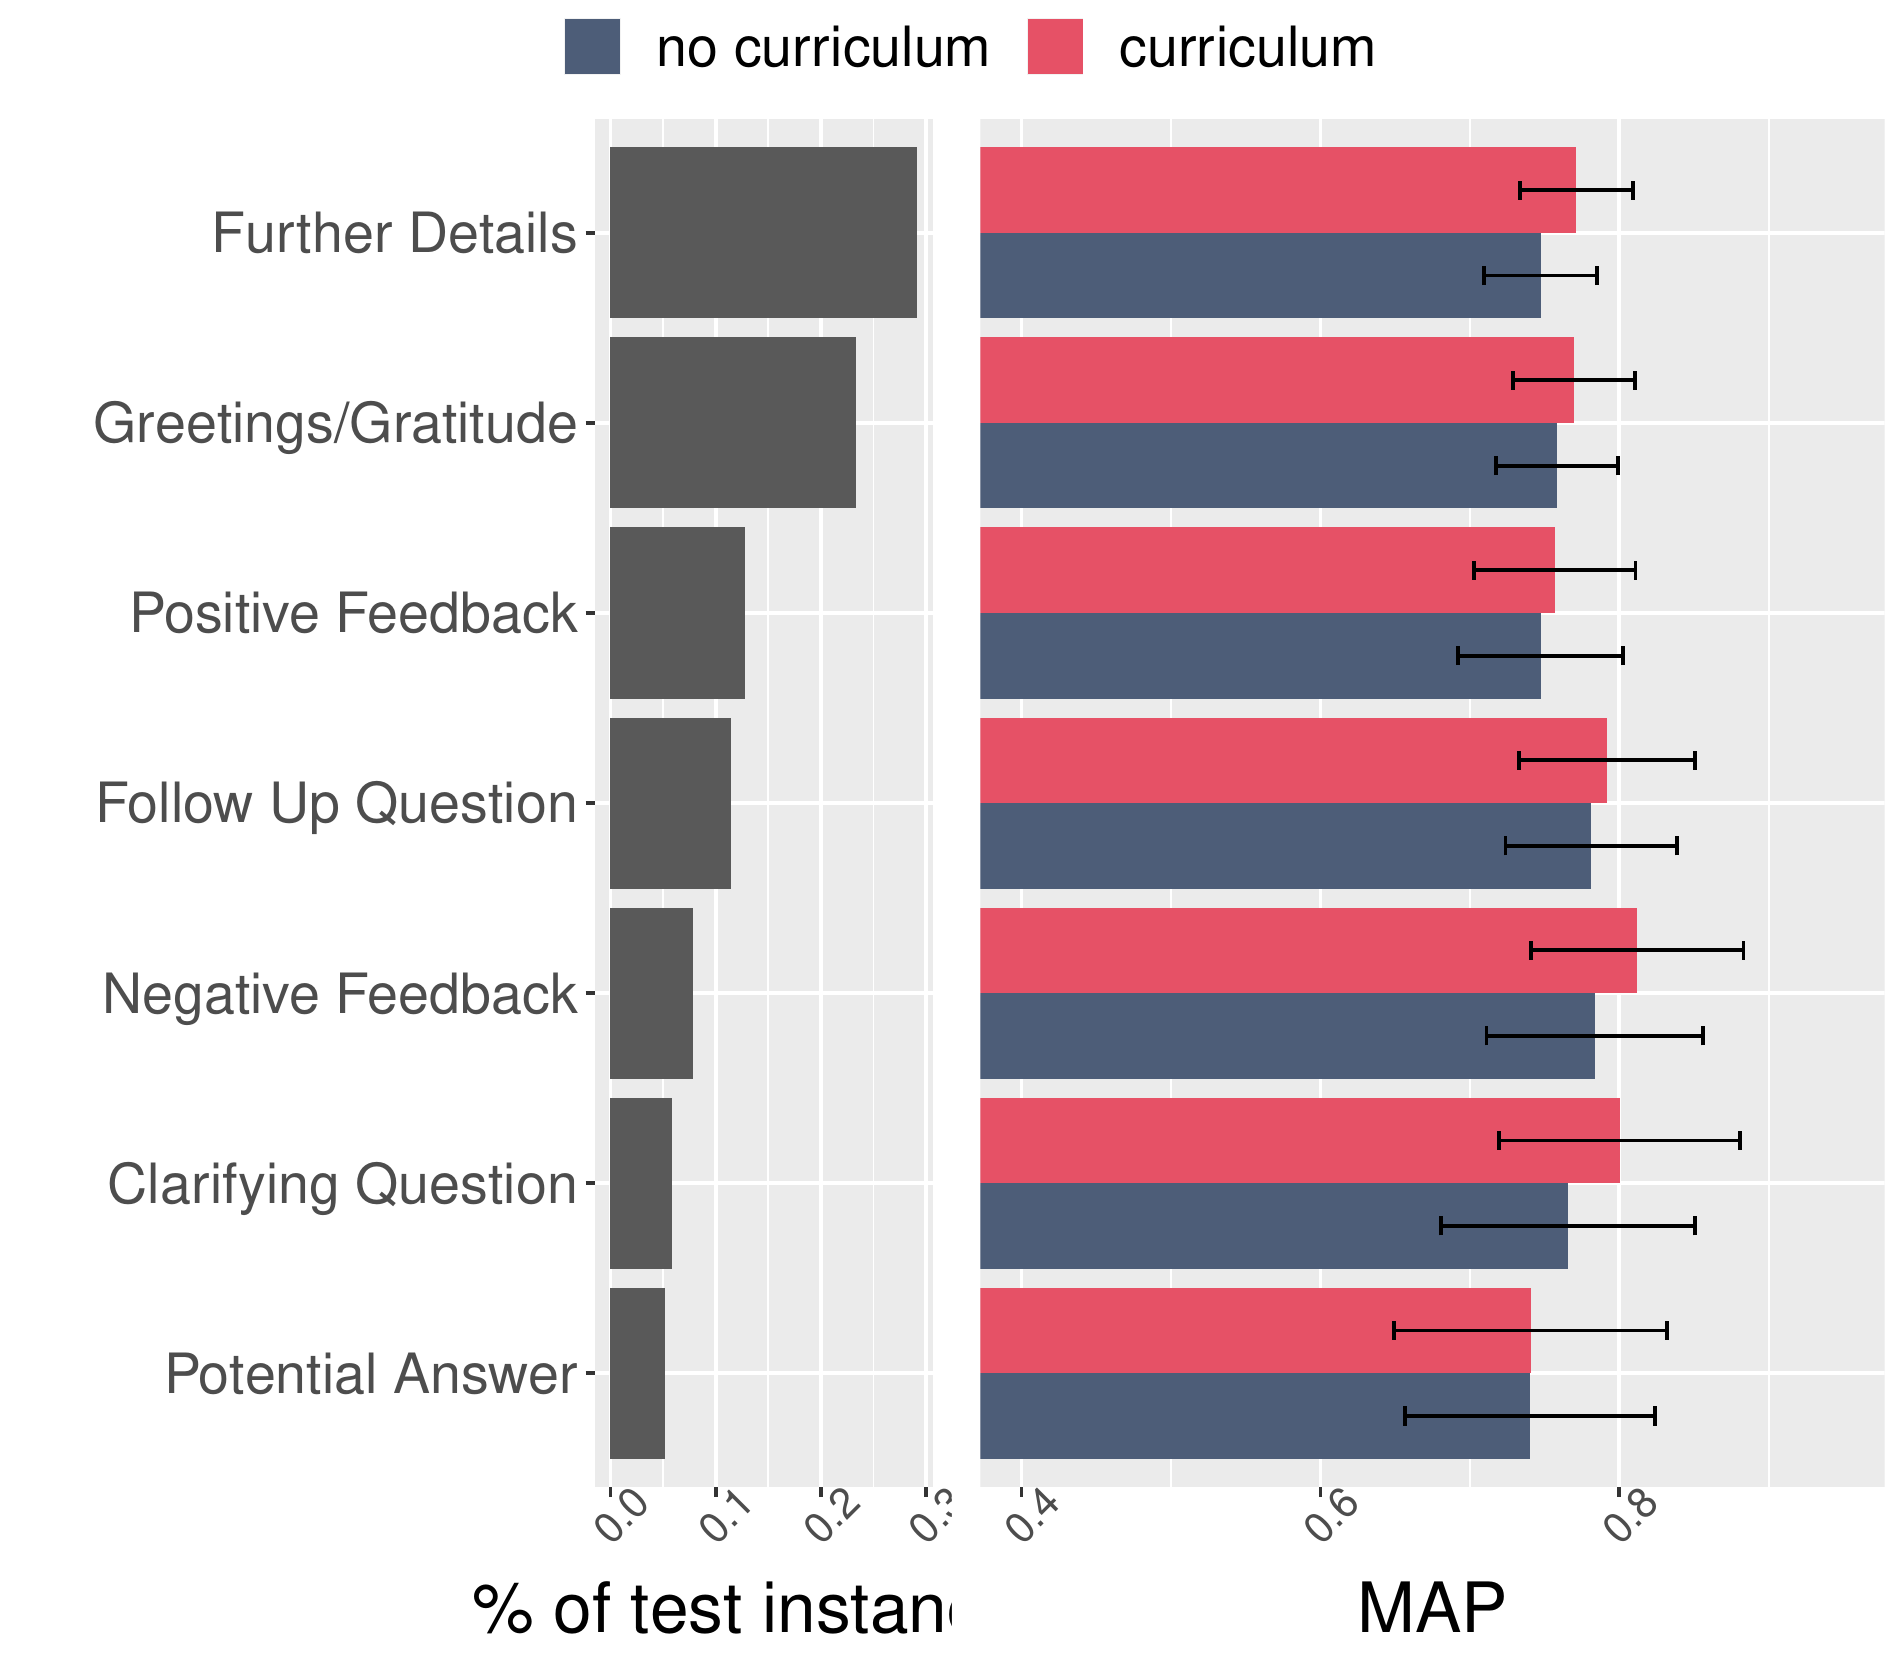}
  \caption{\msdialog{}}
  \label{fig:}
\end{subfigure}%
\begin{subfigure}{.5\textwidth}
  \centering
  \includegraphics[width=1\linewidth]{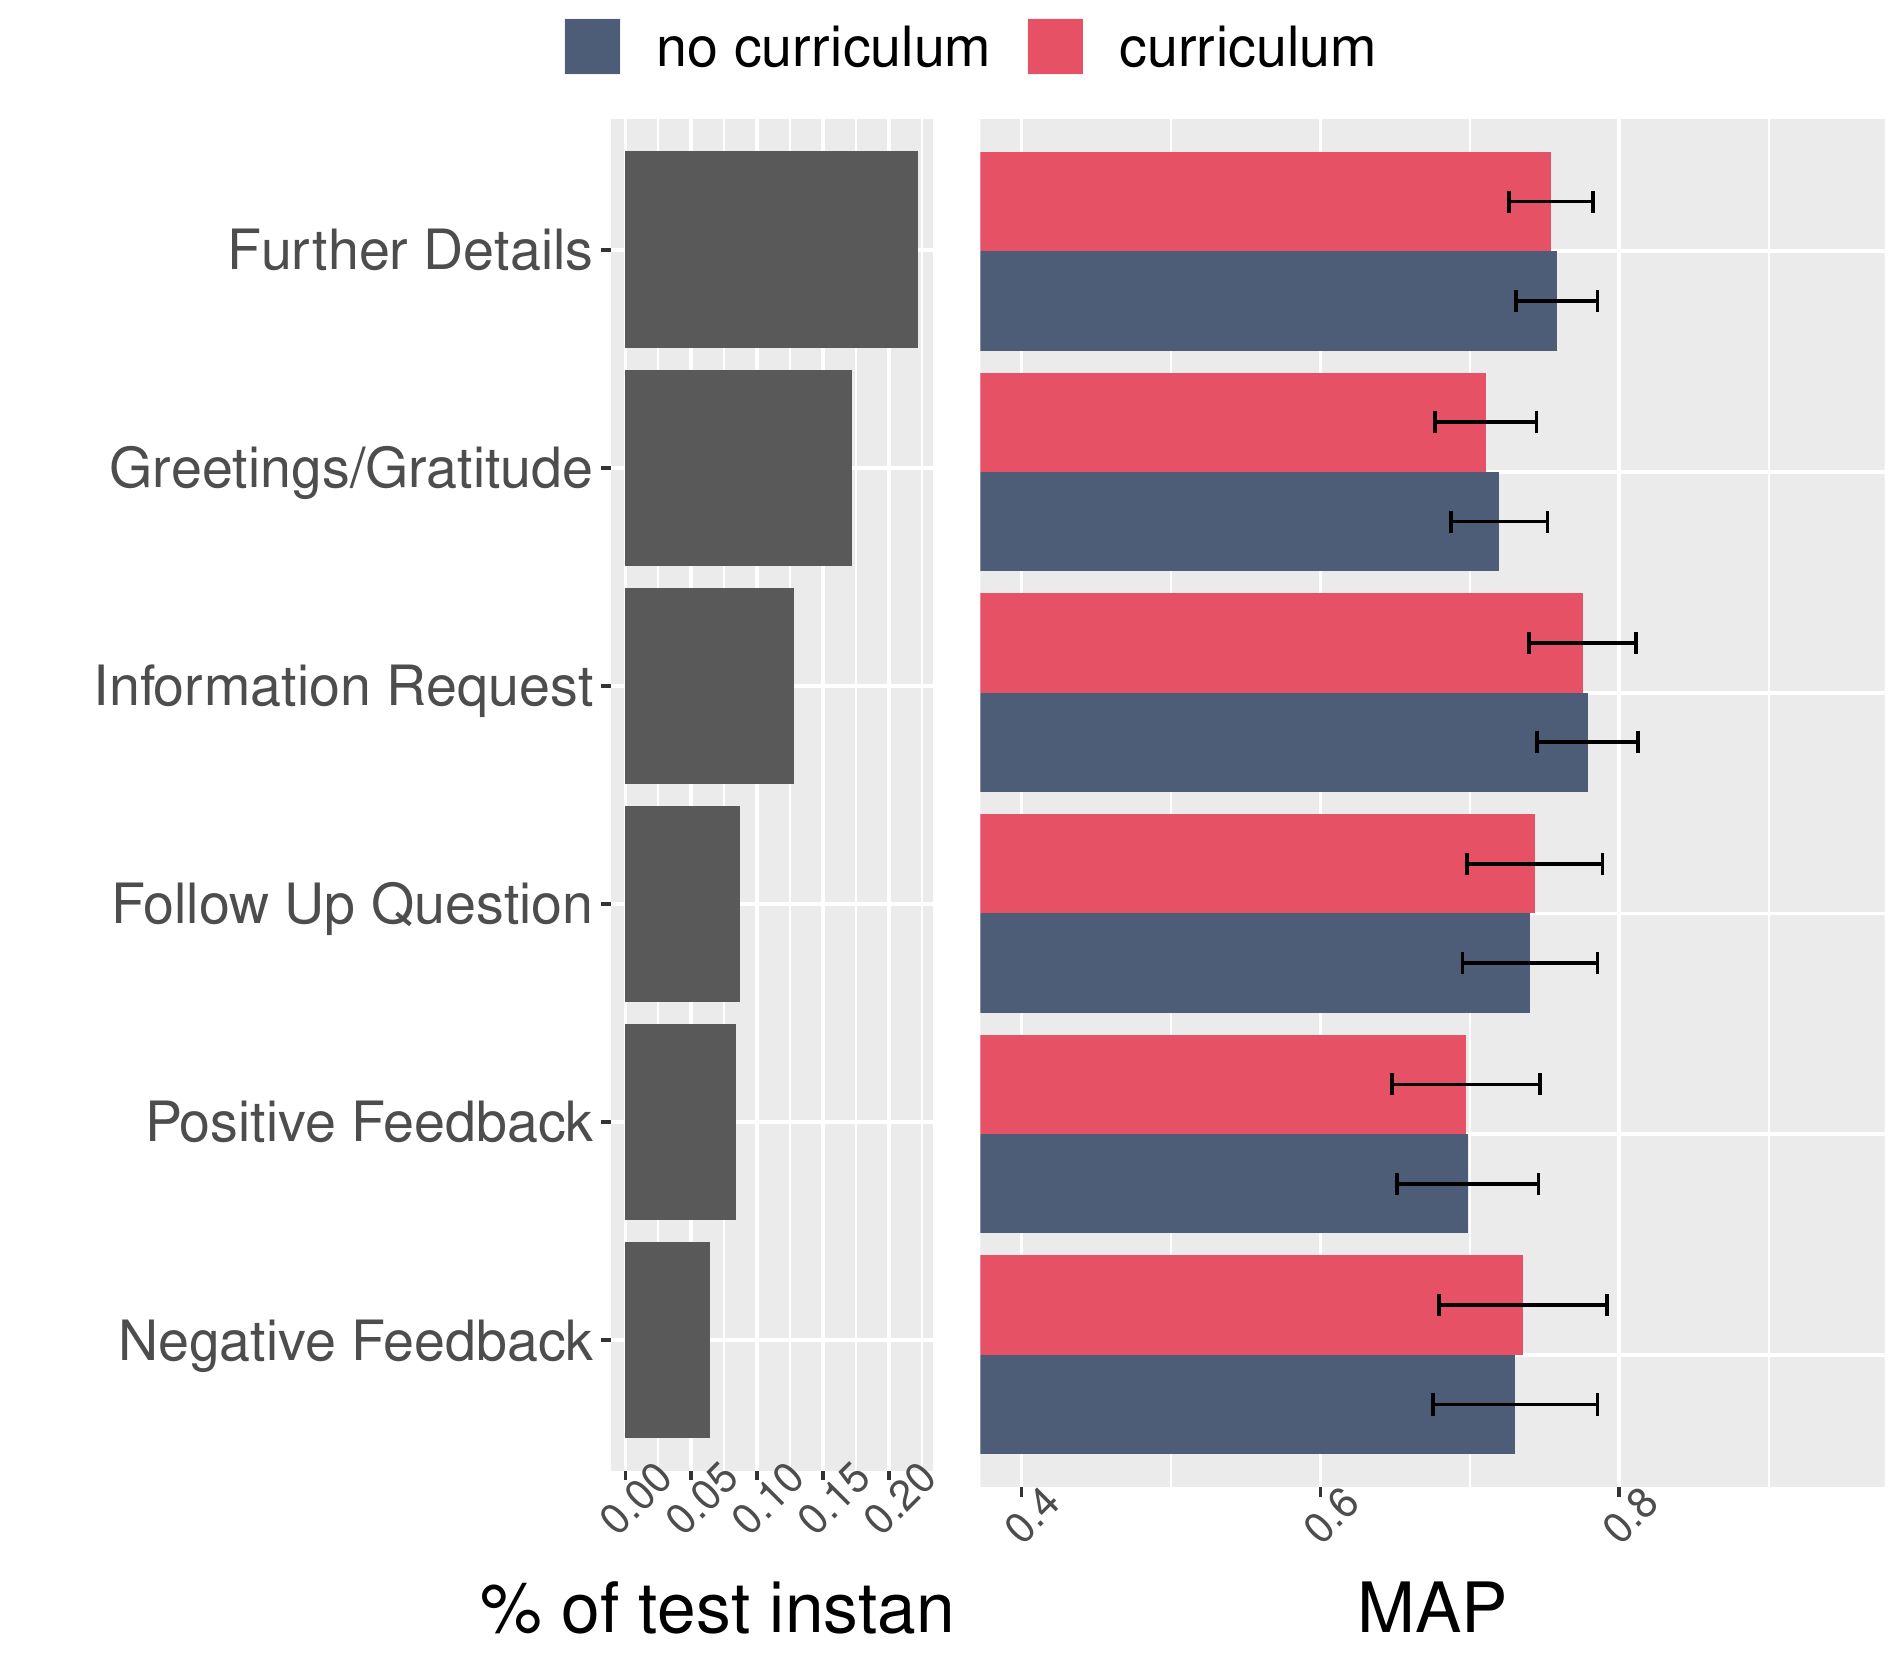}
  \caption{\mantis{}}
  \label{fig:}
\end{subfigure}
\caption{Sensitivity of methods with respect to the intent of the last user utterance. Only $\sim$ 2\% (422) and $\sim$ 9\% (349) of the test instances of \mantis{} and \msdialog{} have user intent labels respectively.}
\label{fig:}
\end{figure}
